# Supplementary material for: Unveiling defect motifs in amorphous GeSe using machine learning interatomic potentials
Source: arXiv:2506.15934 ancillary file (2025-06-19)
Supplement: Supplementary file 1 [file SF_OTS_paper.pdf]

# Supporting Information: Unveiling defect motifs in amorphous GeSe using machine learning interatomic potentials

Minseok Moon,[†] Seungwoo Hwang,[†] Jaesun Kim,[†] Yutack Park,[†] Changho Hong,[*,†] and Seungwu Han[*,†,‡]

†*Department of Materials Science and Engineering and Research Institute of Advanced Materials, Seoul National University, Seoul 08826, Korea*

‡*Korea Institute for Advanced Study, Seoul 02455, Korea*

E-mail: mk01071@snu.ac.kr; hansw@snu.ac.kr

Phone: +82 (02) 880 1541

Table S1: RMSE value of MLIPs on the energy and force of the energy, force, and stress of the train set and test set

| Type | Training set | | | Test set | | |
|---|---|---|---|---|---|---|
| | Energy (meV/atom) | Force (eV/Å) | Stress (kbar) | Energy (meV/atom) | Force (eV/Å) | Stress (kbar) |
| SevenNet | 2.3 | 0.13 | 5.1 | 4.4 | 0.16 | 5.6 |
| MTP | 5.1 | 0.26 | 2.6 | 5.0 | 0.26 | 3.3 |
| BPNN | 7.5 | 0.27 | 5.4 | 9.7 | 0.28 | 6.5 |

Table S2: List of parameters used for atom-centered symmetry functions for each element.

| SF type | $e_c$ | $e_1$ | $e_2$ | $r_c$ (Å) | $s$ | $\lambda$ | $\zeta$ | # of SFs |
|---|---|---|---|---|---|---|---|---|
| $G^2$ | Ge, Se | Ge, Se | – | 8.0 | 0.001214, 0.007284<br>0.015782, 0.027032<br>0.043869, 0.071421<br>0.114987, 0.204264<br>0.357106, 0.714213 | – | – | 20 |
| $G^4$ | Ge, Se | Ge, Se | Ge, Se | 8.0 | 0.000357, 0.010621<br>0.033569, 0.089277 | 1, 2, 4 | -1, 1 | 72 |

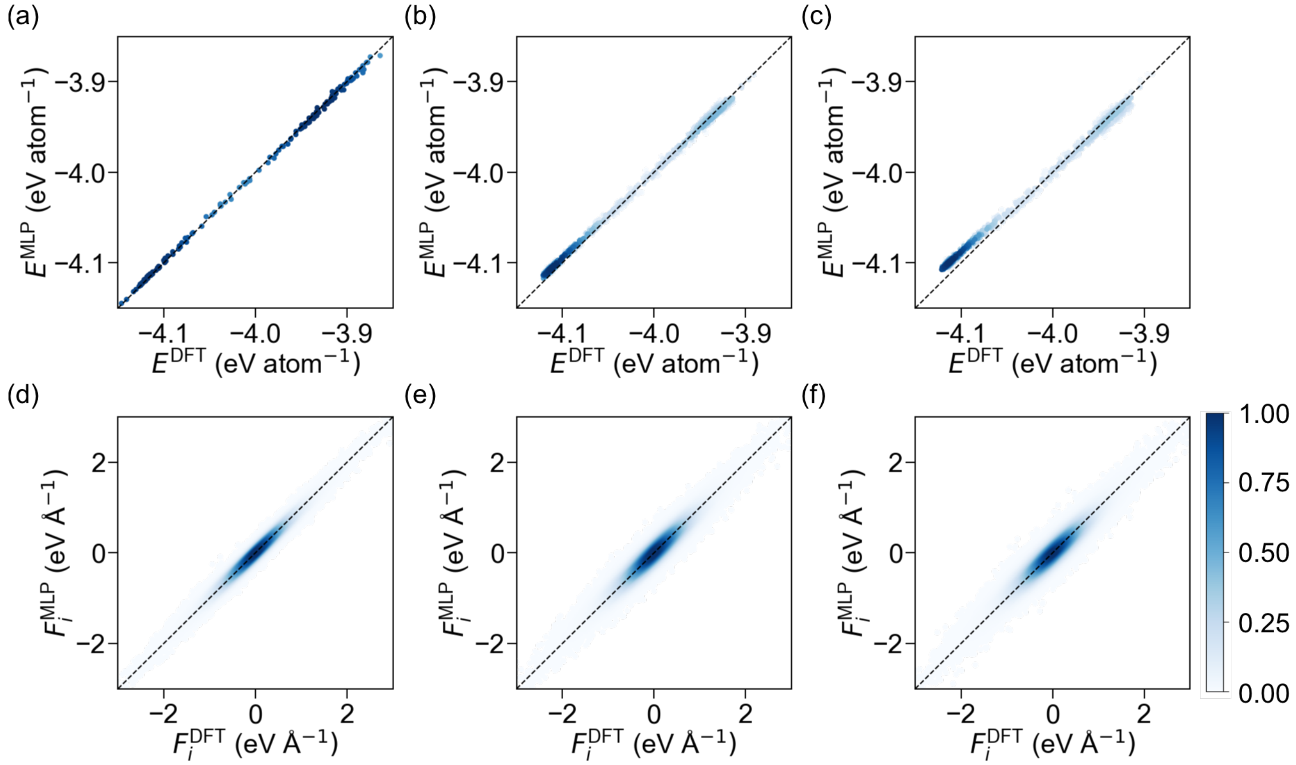


Figure S1: Parity plots of energy (a–c) and atomic force (d–f) values evaluated by DFT versus MLIPs for the test set. The energies evaluated by SevenNet, MTP, and BPNN are shown in (a), (b), and (c), respectively. The atomic forces evaluated by SevenNet, MTP, and BPNN are shown in (d), (e), and (f), respectively. Data points are colored by kernel density estimation (KDE) density values, indicated by the color bar on the right.

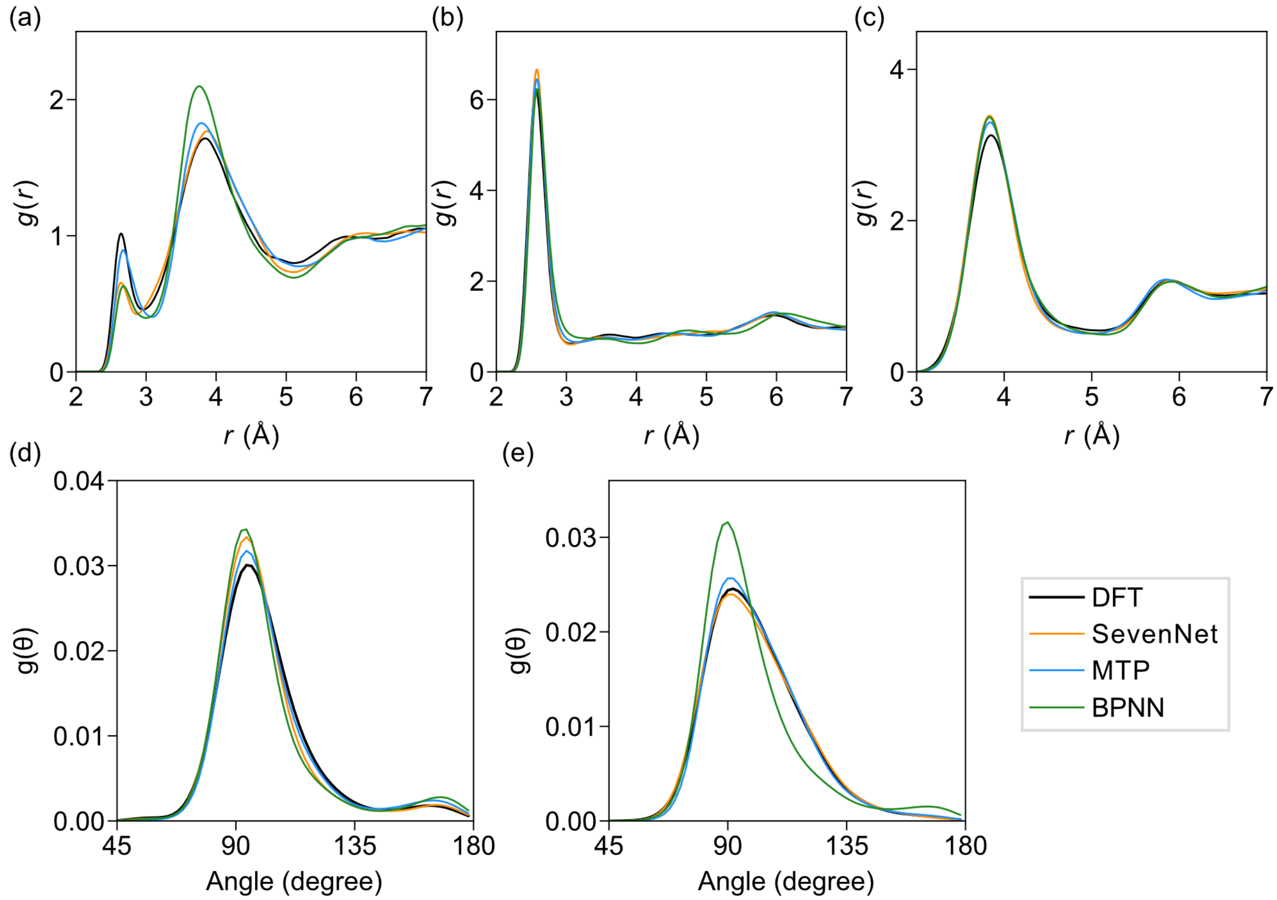


Figure S2: Structural properties of the amorphous phase of GeSe. (a–c) Partial RDFs (a) Ge–Ge, (b) Ge–Se, (c) Se–Se of amorphous GeSe at 300 K. (d–e) Partial ADFs computed with a 3 Å cutoff for (d) Ge total, (e) Se total of amorphous GeSe at 300 K. The black, orange, blue, and green lines represent the results of DFT, SevenNet, MTP, and BPNN, respectively.

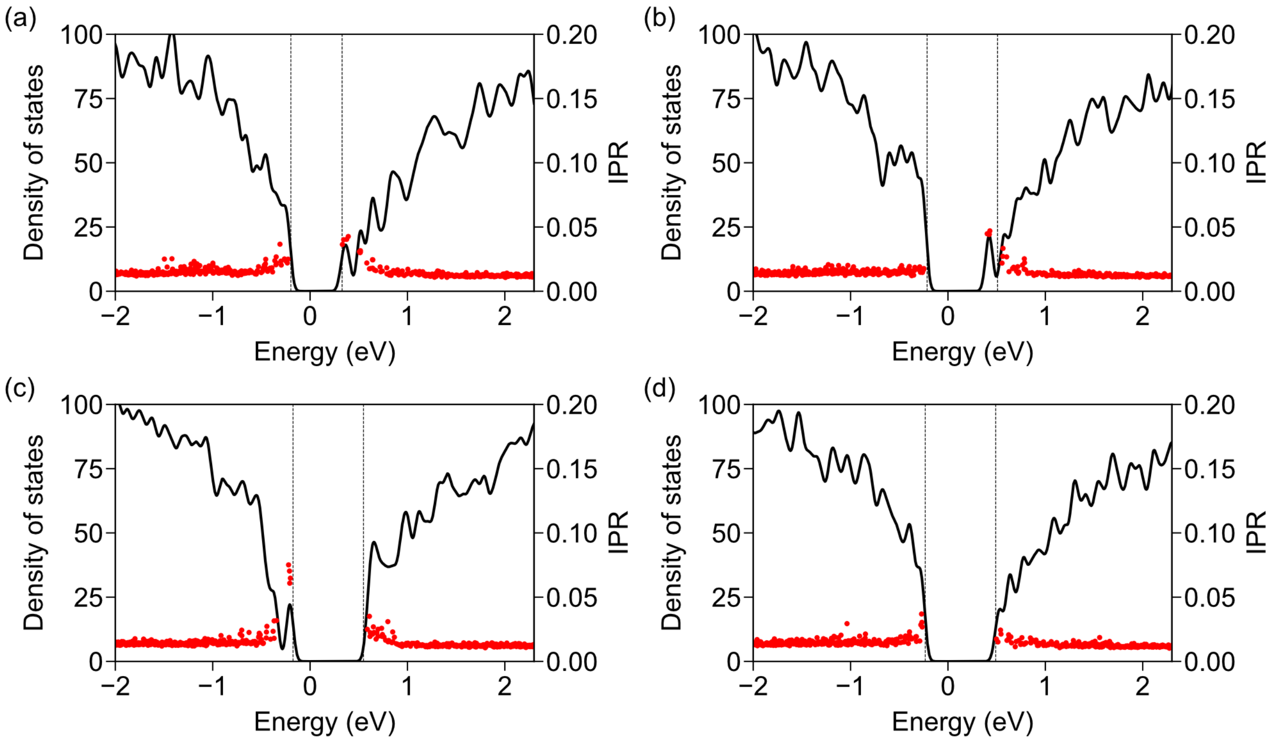


Figure S3: (a–d) Electronic DOS (black lines) and IPR (red dots) of amorphous structures generated by DFT. The dotted lines denote the mobility gap in each DOS plot. Each electronic structure is computed with DFT single point calculation for an amorphous configuration obtained from an independent melt–quench simulation with DFT.

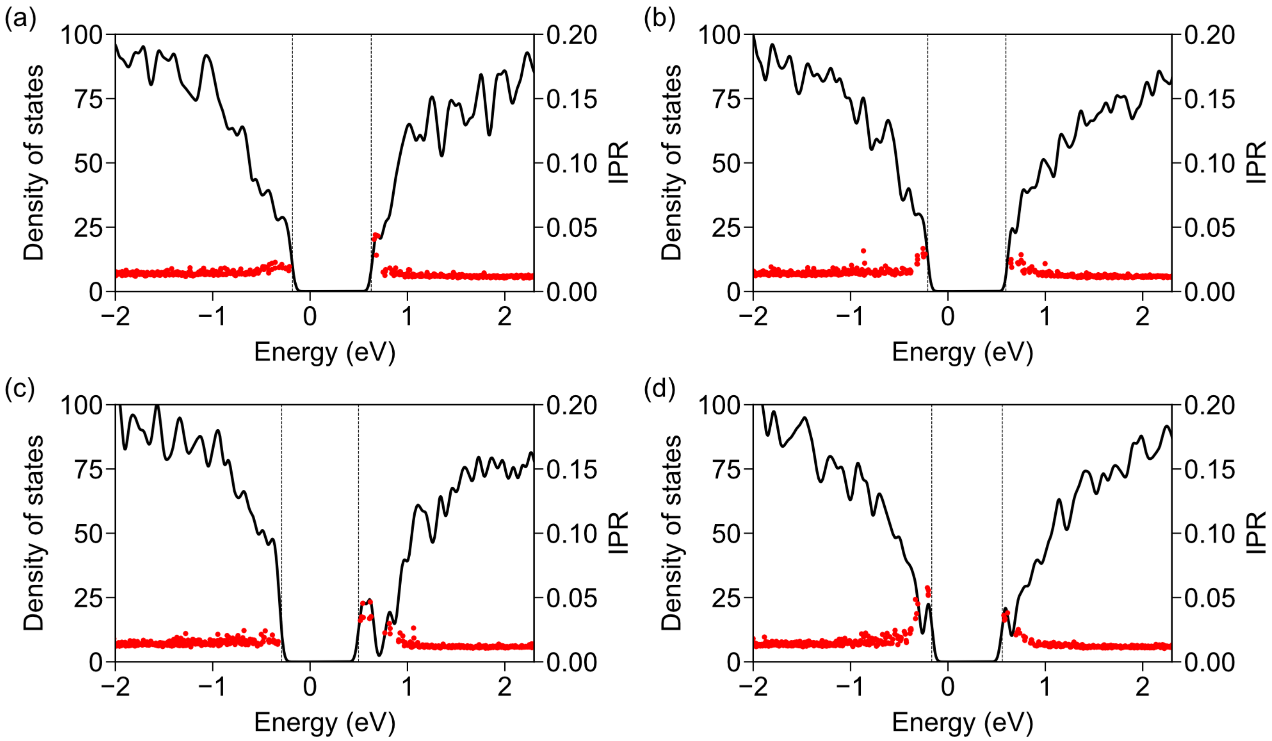


Figure S4: (a–d) Electronic DOS (black lines) and IPR (red dots) of amorphous structures generated by SevenNet. The dotted lines indicate the mobility gap in each DOS plot. Each electronic structure is computed with DFT single point calculation for an amorphous configuration obtained from an independent melt–quench simulation with SevenNet potential.

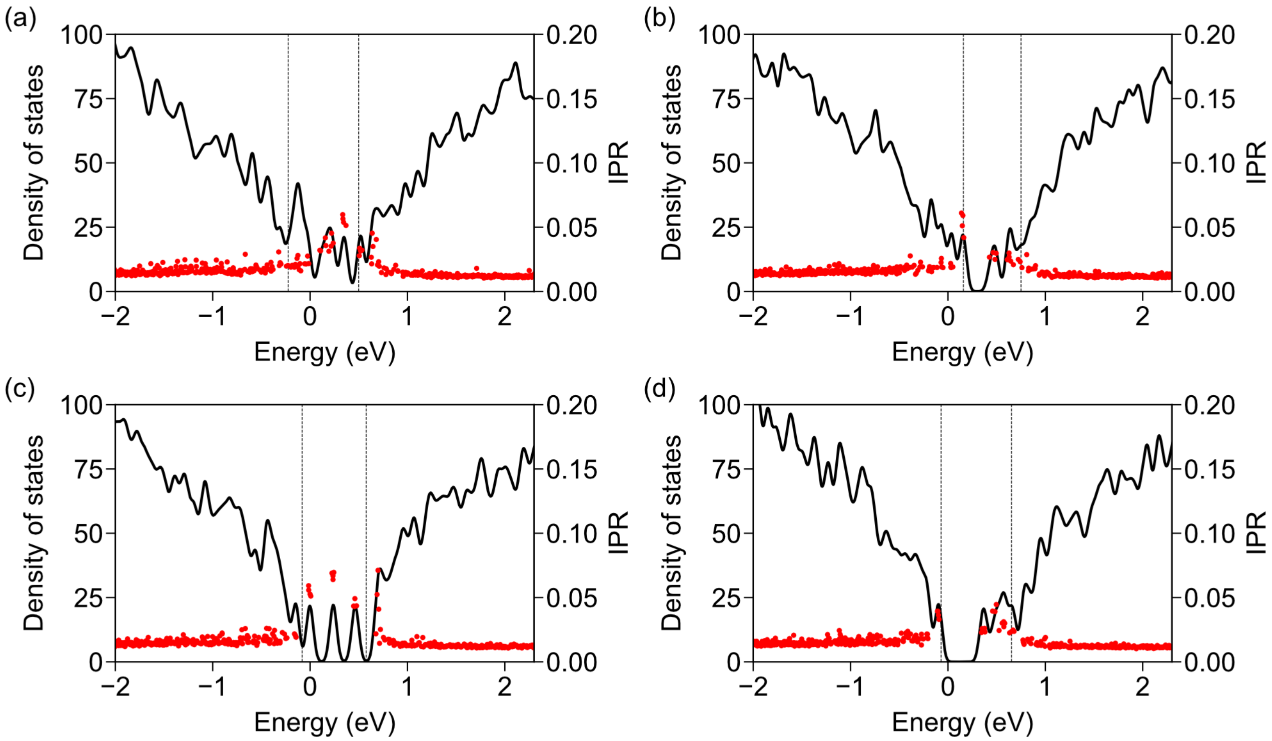


Figure S5: (a–d) Electronic DOS and IPR of amorphous structures generated by MTP. The dotted lines show the mobility gap in each DOS plot. Each electronic structure is computed with DFT single point calculation for an amorphous configuration obtained from an independent melt–quench simulation with MTP potential.

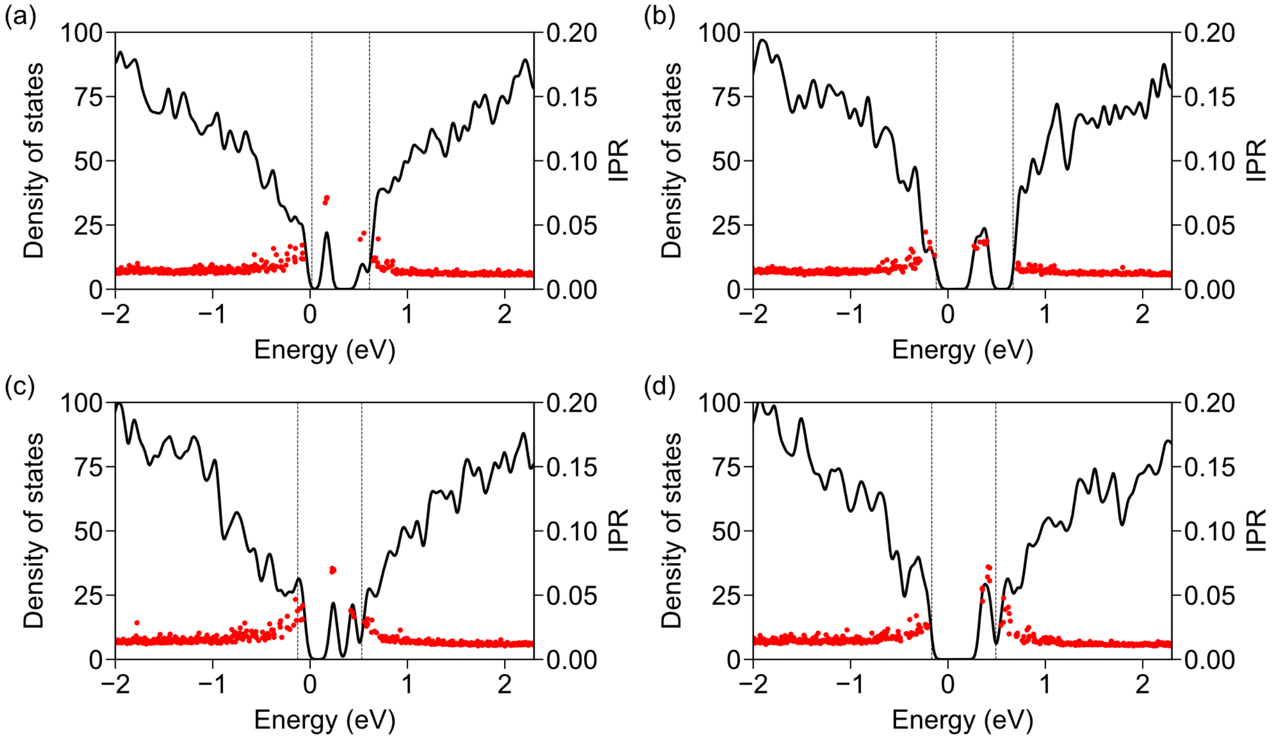


Figure S6: (a–d) Electronic DOS (black lines) and IPR (red dots) of amorphous structures generated by BPNN. The dotted lines denote the mobility gap in each DOS plot. Each electronic structure is computed with DFT single point calculation for an amorphous configuration obtained from an independent melt–quench simulation with BPNN potential.

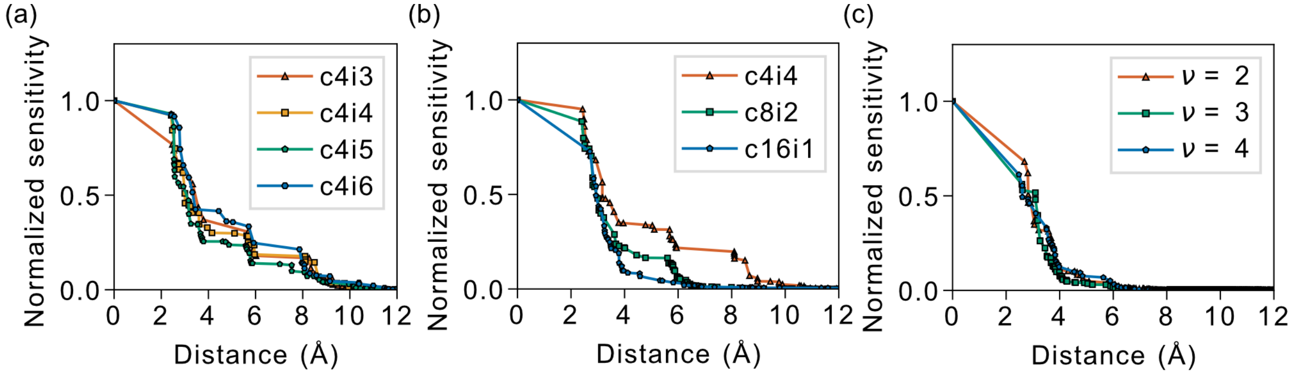


Figure S7: Distance dependence of the SevenNet $S_{(u,v)}$ metric. (a) SevenNet models with a fixed 4 Å cutoff and 3, 4, 5, or 6 interaction layers are shown in blue, orange, green, and red, respectively. (b) Single-communication SevenNet models with cutoff distances of 8, 12, and 16 Å are shown in orange, green, and blue, respectively. (c) Single-communication SevenNet models with maximum correlation orders of 2, 3, and 4 are shown in orange, green, and blue, respectively. For models with fewer than three interaction layers (as in panels b and c), self-tensor products were used to guarantee the minimum multi-atom interaction order.

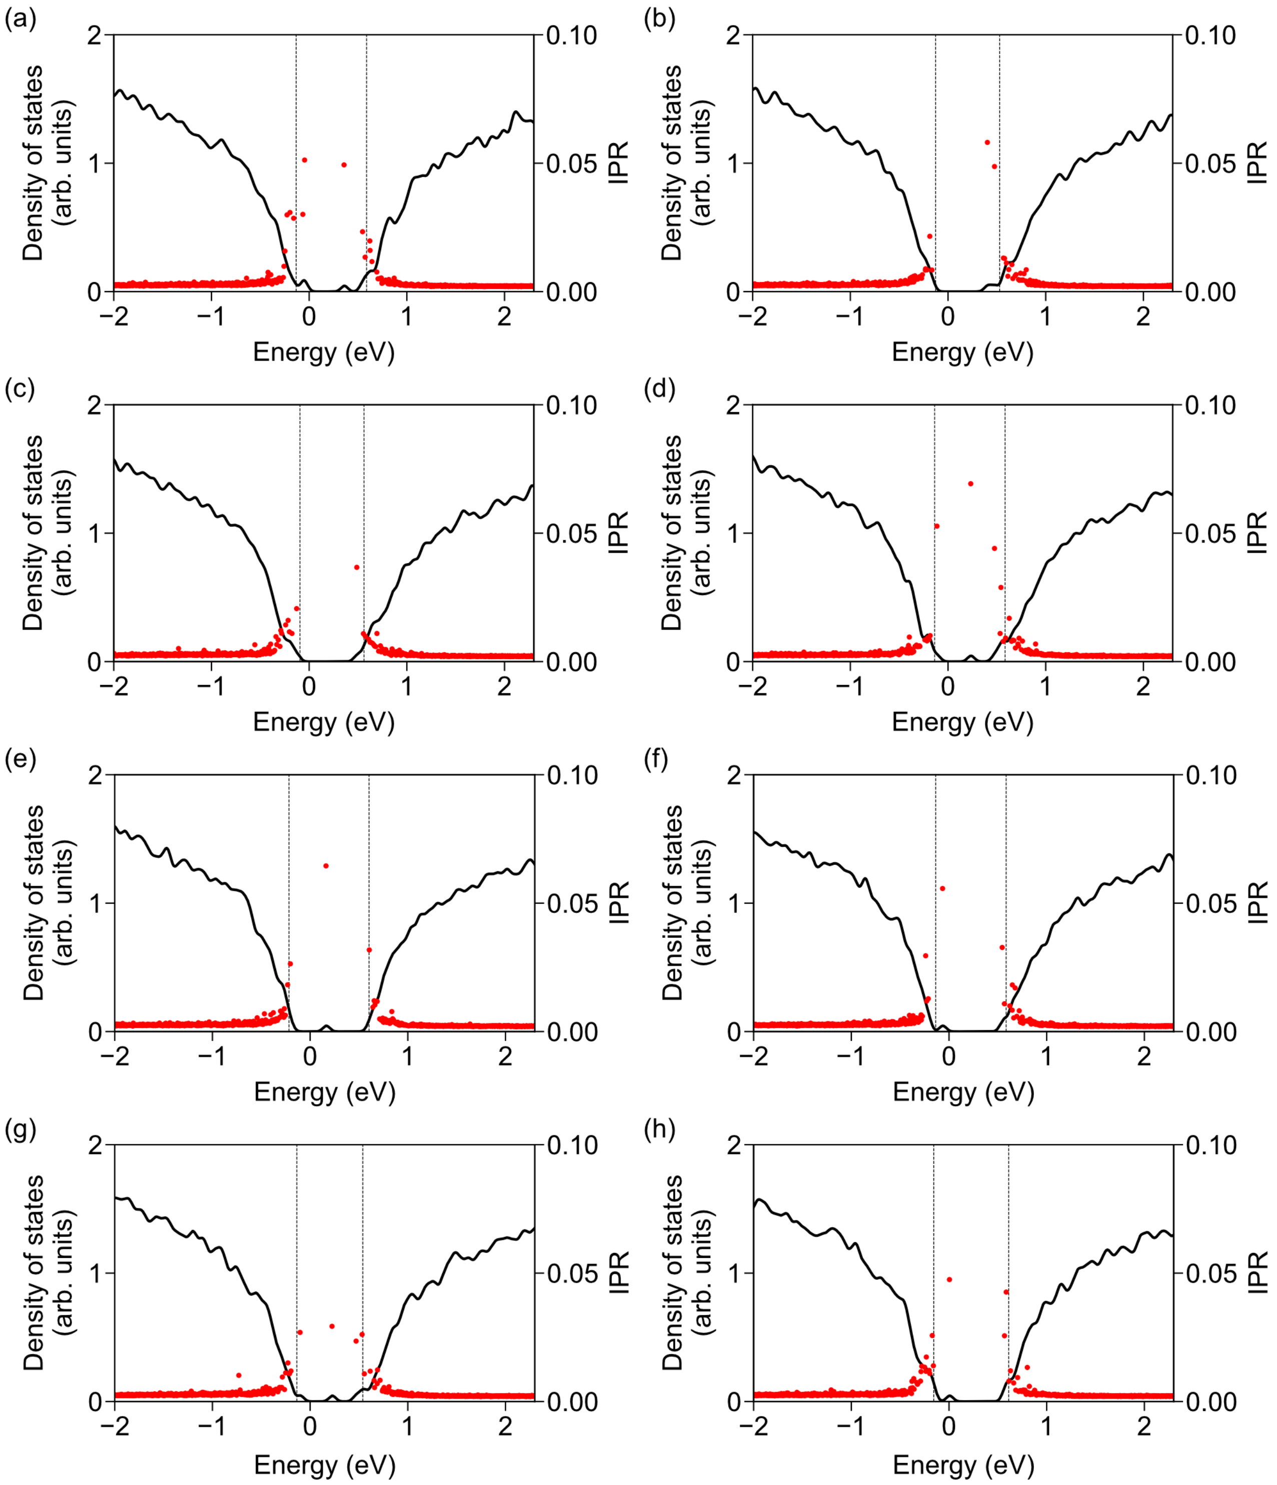


Figure S8: (a–h) Electronic DOS (black lines) and IPR (red dots) of large amorphous structures generated by SevenNet potential. (run1 – run8) The dotted lines denote the mobility gap in each DOS plot. Each electronic structure is computed with DFT single point calculation for an amorphous configuration obtained from an independent melt–quench simulation with SevenNet potential.

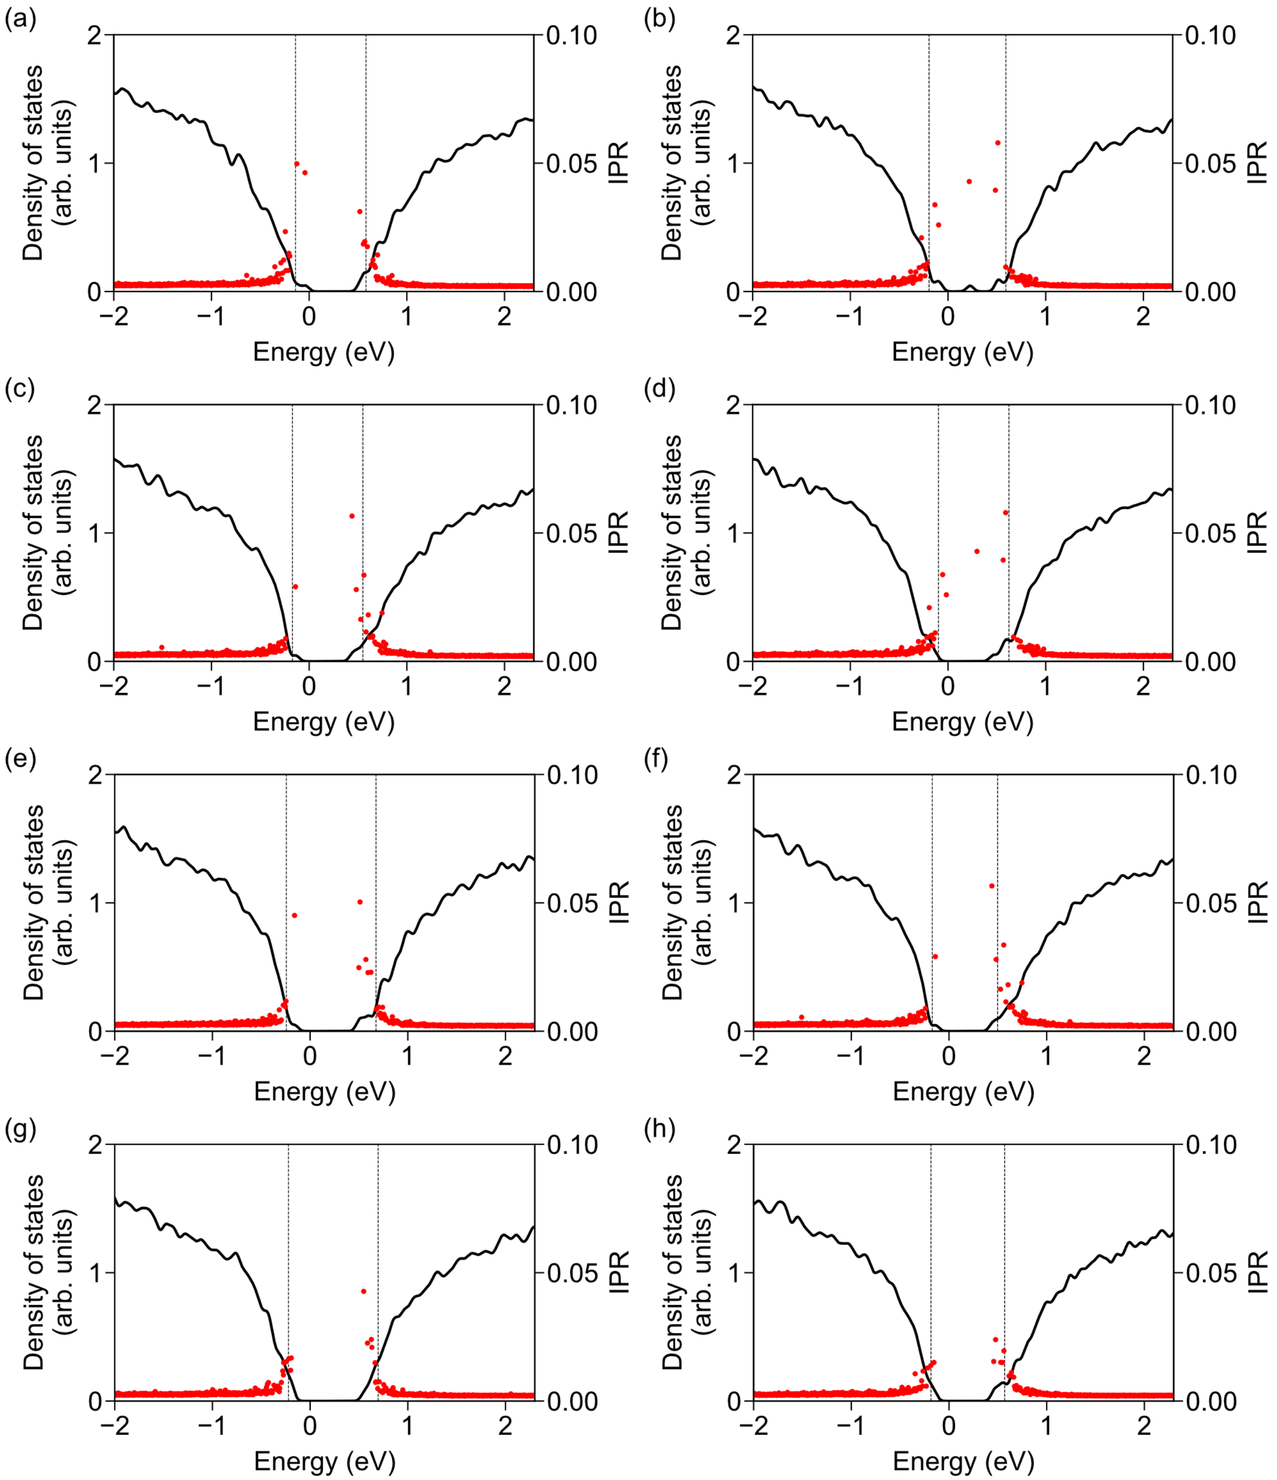


Figure S9: (a–h) Electronic DOS (black lines) and IPR (red dots) of large amorphous structures generated by SevenNet potential. (run9 – run16) The dotted lines denote the mobility gap in each DOS plot. Each electronic structure is computed with DFT single point calculation for an amorphous configuration obtained from an independent melt–quench simulation with SevenNet potential.

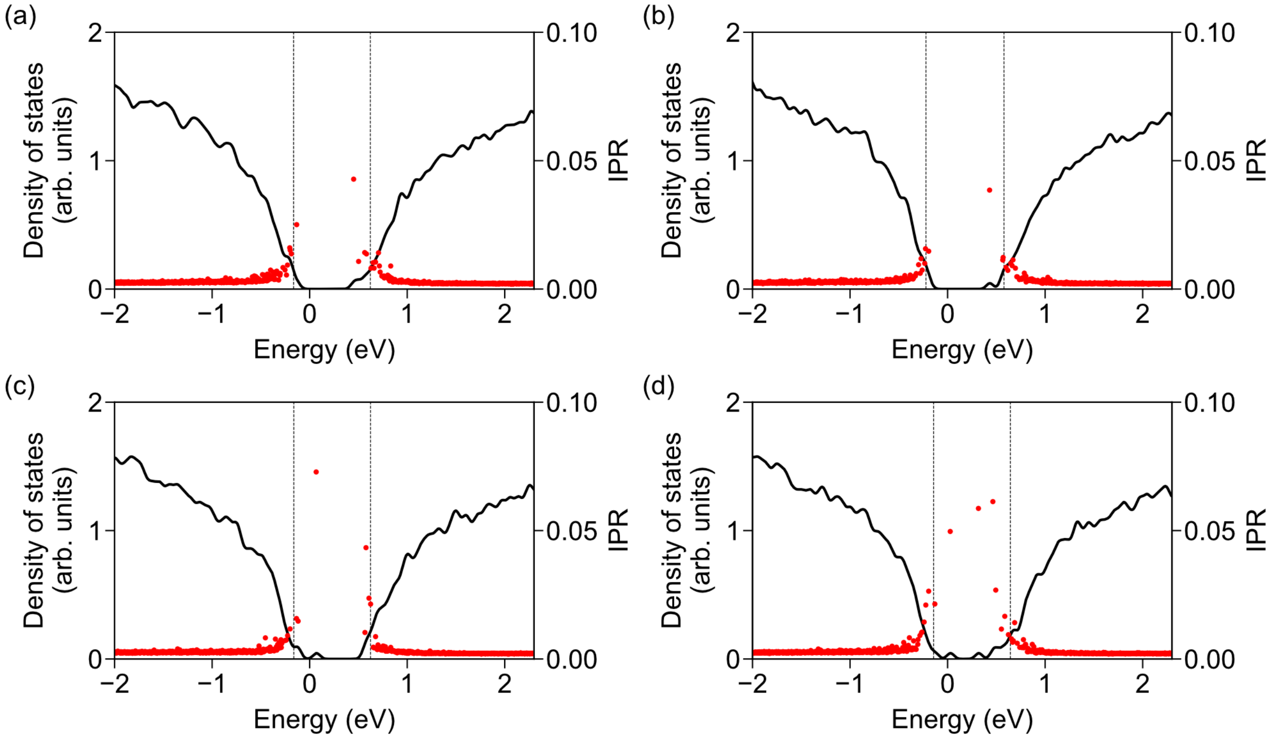


Figure S10: (a–d) Electronic DOS (black lines) and IPR (red dots) large amorphous structures generated by SevenNet potential. (run17 – run20) The dotted lines denote the mobility gap in each DOS plot. Each electronic structure is computed with DFT single point calculation for an amorphous configuration obtained from an independent melt–quench simulation with SevenNet potential.

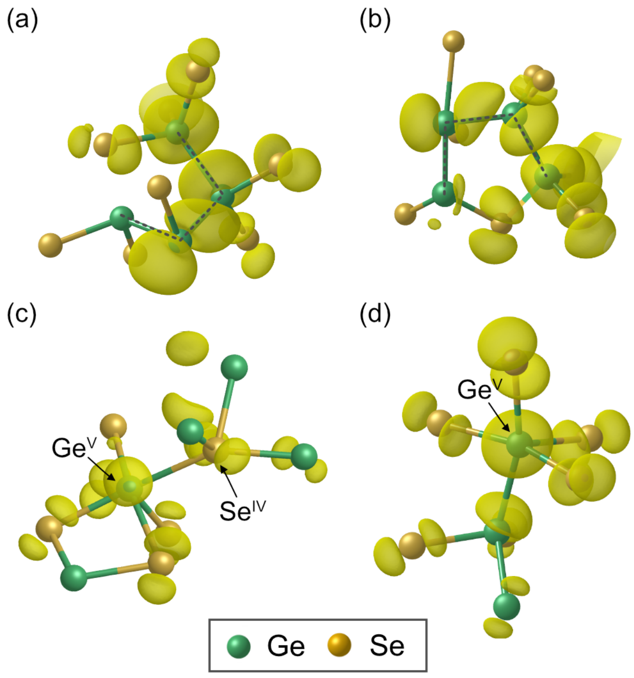


Figure S11: (a,b) Partial charge-density distributions of conduction band tail states in large amorphous GeSe structures generated by the SevenNet model, localized on a Ge-chain motif with less aligned angle. The gray dashed line highlights the Ge chain. (c,d) Partial charge-density distributions of valence band tail states in large amorphous GeSe structures generated by the SevenNet model, localized on an overcoordinated Ge-chain motif with less Peierls distortion ratio. Only atoms contributing to the localized charge density are shown.

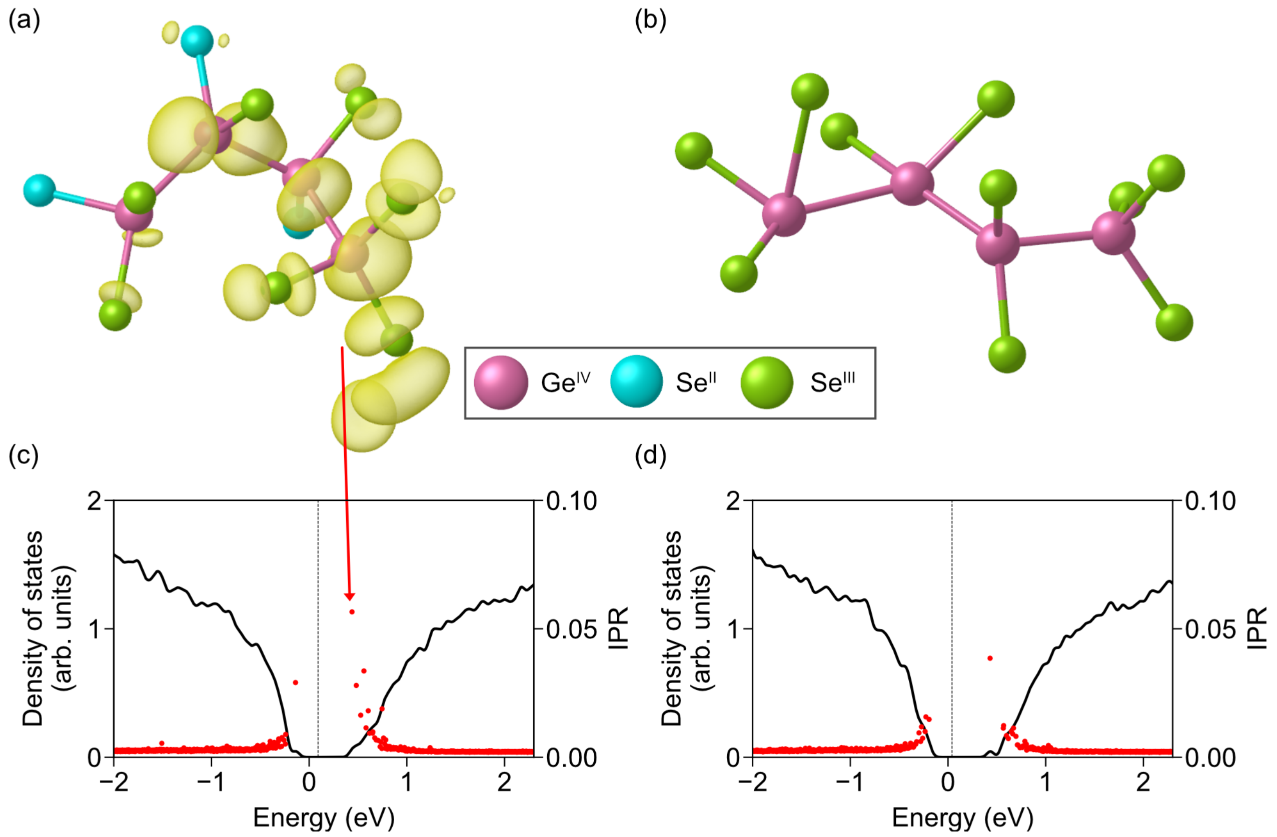


Figure S12: (a) Partial charge-density distributions of mid-gap defect states in large amorphous GeSe structures generated by the SevenNet model, localized on a Ge-chain motif linked by two-coordinate Se atoms. (b) Atomic structures of Ge-chain motifs capped with three-coordinate Se atoms that do not host localized mid-gap states. Only atoms contributing to the localized charge density are shown. (c, d) Corresponding electronic density of states (DOS) and inverse participation ratio (IPR) for the structures in (a) and (b), respectively. Red arrows in the DOS panels indicate the energy levels from which the charge distributions in (a) are extracted.
